# Supplementary material for: MTEB-French: Resources for French Sentence Embedding Evaluation and Analysis
Source: arXiv:2405.20468 source file (2024-06-17)
Supplement: Supplementary file 1 [file datasets_appendix.tex]

\subsection{Bitext mining}

\paragraph{Diabla}
This dataset contains a set of informal written dialogues for evaluating English-French machine translation on informal texts \citep{bawden_DiaBLa:-A-Corpus-of_2021}. The dataset contains over 5700 text pairs extracted from 144 dialogues, along with their machine translation (MT) and the annotations of the MT quality produced by the dialogue participants themselves.

\paragraph{Flores}
Flores is a benchmark dataset for machine translation between English and low-resource languages \citep{nllb2022} \citep{FLORES-101} \citep{Nepali-English}. The newer version, FLORES-200, consists of translations from 842 distinct web articles, totaling 3001 sentences. We use the French subset of this dataset, in other words, the English-to-French translated texts which contains approximately 997 samples.

\subsection{Retrieval}

\paragraph{Alloprof}
This question-answering dataset is collected from Alloprof, a Quebec-based primary and high-school help website. It contains almost 30k question-answer pairs, spread over a variety of school subjects \citep{lef23}. More than half of the answers also contain a link to a reference page addressing the question’s topic. The dataset has been cleaned and formatted for the retrieval task: only French questions mentioning a reference page were kept, and all reference pages have been consolidated as a corpus dataset.
