# Supplementary material for: MTEB-French: Resources for French Sentence Embedding Evaluation and Analysis
Source: arXiv:2405.20468 source file (2024-06-17)
Supplement: Supplementary file 2 [file appendix_bge.tex]

For \emph{BAAI/BGE-m3} and \emph{manu/bge-m3-custom-fr} we used \emph{FalgEmbeddings} library and loaded both models with a \emph{fp16} precision. We provide the code used for evaluation below:

\begin{lstlisting}[frame=single,linewidth=\columnwidth,breaklines=true,language=Python]
def encode_documents(self, input: Documents) -> Embeddings:
   embeddings = self.model.encode(
       input,
       max_length=self.max_token_length,
       return_dense=True,
       return_sparse=False, 
       return_colbert_vecs=False
   )
    return embeddings['dense_vecs'].tolist()
\end{lstlisting}
